# Supplementary material for: HopsFS: Scaling Hierarchical File System Metadata Using NewSQL Databases
Source: arXiv:1606.01588 source file (2017-02-22)
Supplement: Supplementary file 1 [file appendix.tex]

\iffalse
\begin{table}[ht]
	\centering
    \begin{tabular}{ | l | l | l | }
\hline
	\textbf{Column Name} & \textbf{Type} & \textbf{Max Size} \\ \hline
	under\_construction & bit(1) & * \\ \hline
	client\_node & varchar(100) & 104 \\ \hline
	parent\_id & int(11) & 4 \\ \hline
	dir & bit(1) & * \\ \hline
	subtree\_lock\_owner & bigint(20) & 8 \\ \hline
	symlink & varchar(3000) & 3012 \\ \hline
	inode\_id & int(11) & 4 \\ \hline
	generation\_stamp & int(11) & 4 \\ \hline
	modification\_time & bigint(20) & 8 \\ \hline
	client\_machine & varchar(100) & 104 \\ \hline
	access\_time & bigint(20) & 8 \\ \hline
	name & varchar(3000) & 3012 \\ \hline
	permission & Varbinary(128) & 132 \\ \hline
	quota\_enabled & bit(1) & * \\ \hline
	subtree\_locked & bit(1) & * \\ \hline
	client\_name & varchar(100) & 104 \\ \hline
	header & bigint(20) & 8 \\ \hline
	primary key index & hash index & 16 \\ \hline
	inode\_idx & btree index & 16 \\ \hline
	Row Size  &  & 6512\  \\ \hline
	Row Size with overhead &  & 6586 \\ \hline
	* all bit fields \\ are compacted \\ into a 4 byte word &  &  \\ \hline
\end{tabular}
\caption{Inode table memory consumption.}
\label{inode_table}
\end{table}


\begin{table}[ht]
	\centering
    \begin{tabular}{ | l | l | l | }
\hline
	\textbf{Column Name} & \textbf{Type} & \textbf{Max Size} \\ \hline
	time\_stamp & bigint(20) & 8 \\ \hline
	primary\_node\_index & int(11) & 4 \\ \hline
	num\_bytes & bigint(20) & 8 \\ \hline
	block\_recovery\_id & bigint(20) & 8 \\ \hline
	block\_index & int(11) & 4 \\ \hline
	inode\_id & int(11) & 4 \\ \hline
	block\_id & bigint(20) & 8 \\ \hline
	block\_under\_construction\_state & int(11) & 4 \\ \hline
	generation\_stamp & bigint(20) & 8 \\ \hline
	primary key index & hash index & 16 \\ \hline
	Row Size &  & 72 \  \\ \hline
	Row Size with overhead &  & 114 \  \\ \hline
\end{tabular}
\caption{Block table memory consumption.}
\label{block_table}
\end{table}

\begin{table}[ht]
	\centering
    \begin{tabular}{ | l | l | l | }
\hline
	\textbf{Column Name} & \textbf{Type} & \textbf{Max Size} \\ \hline
	inode\_id & int(11) & 4 \\ \hline
	block\_id & bigint(20) & 8 \\ \hline
	primary key index & hash index & 16 \\ \hline
	Row Size &  & 28 \  \\ \hline
	Row Size with overhead &  & 66 \  \\ \hline
\end{tabular}
\caption{Block lookup table memory consumption.}
\label{block_lookup_table}
\end{table}

\begin{table}[h]
	\centering
    \begin{tabular}{ | l | l | l | }
\hline
	\textbf{Column Name} & \textbf{Type} & \textbf{Max Size} \\ \hline
	storage\_id & int(11) & 4 \\ \hline
	replica\_index & int(11) & 4 \\ \hline
	inode\_id & int(11) & 4 \\ \hline
	block\_id & bigint(20) & 8 \\ \hline
	primary key index & hash index & 16 \\ \hline
	storage\_idx & btree index & 16 \\ \hline
	Row Size &  & 52 \\ \hline
	Row Size with overhead &  & 90 \  \\ \hline
\end{tabular}
\caption{Replica table memory consumption.}
\label{replica_table}
\end{table}
\fi
